# Supplementary material for: Analysis of a blockchain protocol based on LDPC codes
Source: arXiv:2202.07265 source file (2022-04-30)
Supplement: Supplementary file 1 [file Appendix.tex]

\subsection*{Proof of Lemma \ref{lem:merkle}}

We first prove the lower bound.
Let $P$ denote the probability that $\tilde{\6a}\neq \6a$ leads to a Merkle tree where the penultimate layer (\ie, the one with label $s-1$) is equal to the one in the tree constructed from $\6a$.
The probability that the two trees have the same root is obtained as
$$P + (1-P)2^{-\ell_\hash} = 2^{-\ell_\hash} + P\left(1-2^{-\ell_\hash}\right)\geq 2^{-\ell_\hash}.$$
The above chain of inequalities proves the lower bound.

To derive the upper bound, we employ an inductive reasoning.
For the tree constructed from $\6a$, we are going to use $h_{j}^{(i)}\in D$ to indicate the value of the $j$-th leaf in the $i$-th layer, and start numbering the layers from $0$.
Since $k = 2^s$, the tree is going to have $s+1$ layers (with labels in $\{0,\ldots,s\}$).
For the tree constructed from $\tilde{\6a}$, we employ an analogous notation, and hence use $\tilde{h}_j^{(i)}$ to denote the value of the $j$-th leaf in the $i$-th layer.
Let us start with the case of $s = 1$ (\ie, with $\6a$ and $\tilde{\6a}$ having only two elements).
The trees constructed from $\6a$ and $\tilde{\6a}$ will have the same root if and only if one of the two following conditions is satisfied: 
\begin{itemize}
    \item[I) ] the base layer is identical, \ie, $\hash(a_0) = h_0^{(0)} = \tilde{h}_0^{(0)} = \hash(\tilde{a_0})$ and $\hash(a_1) = h_1^{(0)} = \tilde{h}_1^{(0)} = \hash(\tilde{a_1})$;
    \item[II) ] the base layer is not identical but the trees have the same root, \ie,  $(h_0^{(0)}, h_1^{(0)})\neq(\tilde h_0^{(0)}, \tilde h_1^{(0)})$ and $\hash(h_0^{(0)}||h_1^{(0)}) = \hash(\tilde h_0^{(0)}||\tilde h_1^{(0)})$.
\end{itemize}
The probability with which the above two conditions are satisfied depends on the number of coordinates in which $\6a$ and $\tilde{\6a}$ differ.
Indeed, if the two vectors differ in two positions, then condition I is satisfied with probability $2^{-2\ell_\hash}$, while condition II is satisfied with probability $(1-2^{-2\ell_\hash})2^{-\ell_\hash}$.
Then, when $\6a$ and $\tilde{\6a}$ differ in two positions, a root collision happens with probability
\begin{align}
\label{eq:pr_distinct}
2^{-2\ell_\hash}+(1-2^{-2\ell_\hash})2^{-\ell_\hash} = 2^{-\ell_\hash}+2^{-2\ell_\hash} - 2^{-3\ell_\hash}.     
\end{align}
If, instead, $\6a$ and $\tilde{\6a}$ differ in just one position, then we have that condition I is satisfied with probability $2^{-\ell_\hash}$ and condition II is satisfied with probability $(1-2^{-\ell_\hash})2^{-\hash}$.
Then, a root collision happens with probability
\begin{align}
\label{eq:pr_one_difference}
2^{-\ell_\hash} + (1-2^{-\ell_\hash})2^{-\ell_\hash}&    = 22^{-\ell_\hash} - 2^{-2\ell_\hash}\\
& = (s+1)2^{-\ell_\hash} - 2^{-2\ell_\hash}.
\end{align}
It is easy to prove that, if $\ell_\hash>1$, then the probability in \eqref{eq:pr_one_difference} is always larger than that expressed in \eqref{eq:pr_distinct}.
Let us now generalize to the case of $s = 2$
To prove the upper bound, we consider
Let $\6a\rand A^k$: because of the ROM, we have that $h$ is uniformly distributed over $D$ (that is, $h\rand D$).
For $\tilde{\6a}\in A^k\setminus\{\6a\}$, we will denote with $\tilde{h}^{(i)}_j$ the $j$-th leaf in the $i$-th layer. If $\tilde{\6a}$ is such that $\mroot(\tilde{\6a}) = \6a$, then one of the following two conditions must be true:

Let us start by considering condition I.
Let $M_i$ denote the number of vectors from $A^k\setminus\{\6a\}$ for which the $i$-th layer is identical to the $i$-th one of $\mathcal M(\6a)$.
The number of vectors yielding to a macth in the root is estimated as
\begin{align*}
N_h = 2^{-\ell_\hash}\left(|A| - M_{s-1}\right) + M_{s-1},    
\end{align*}
since
\begin{itemize}
\item[-] the term $M_{s-1}$ accounts for the vectors giving an equality in the penultimate layer;
\item[-] the term $(|A| - M_{s-1})$ counts the number of vectors where all layers but the last (\textit{i.e.}, the root) are distinct.
\end{itemize}
The above quantity can be bounded as
\begin{align*}
N_h = 2^{-\ell_\hash}|A| + M_{s-1}\left(1-2^{-\ell_\hash}\right)\geq |A|2^{-\ell_\hash},   
\end{align*}
which proves the lower bound.
To prove the upper bound, we make the following considerations:
\begin{itemize}
\item[-] let us consider the base layer of $\mathcal M(\tilde{\6a})$, and consider the number of input vectors for which exactly $w$ out of $k$ leaves are identical.
This number can be estimated as
$$M^{(0)}(w) = |A|\binom{k}{w}\big(2^{-\ell_\hash}\big)^w(1-2^{-\ell_\hash})^{k-w}.$$
For $w = k$, we have two identical tries; notice that
$$M^{(0)}(k) = |A|2^{-k\ell_H}$$
\item[-] 
\item[-] if layers number $i$ in $\mathcal M(\6a)$ and $\mathcal M(\6a')$ differ in $w$ contiguous pairs, the number of vectors which, on average, lead to identical layers is given by
$$2^{s-i-1}$$
\end{itemize}
